# Supplementary material for: APPTeK: Agent-Based Predicate Prediction in Temporal Knowledge Graphs
Source: arXiv:2110.14284 source file (2022-07-21)
Supplement: Supplementary file 1 [file _appendix.tex]

\clearpage
\onecolumn
\section{Related Work - Comparison}
\label{appendix:rel_work_comparison}

Let $e_s$ be the source entity, $e_q$ be the query entity, and $e_t$ be the entity which is explored by an agent at iteration $t$, the MDP environment and policy networks of these methods are summarized in table \ref{tab:scoring_fncs}, where for the inference, \emph{MINERVA}, \emph{M-Walk} and \emph{CPL} use binary rewards. For the policy networks, \emph{DeepPath} uses fully-connected network, the extractor for textual information of \emph{CPL} employs convolutional neural net, while the rest uses recurrent neural networks. 

For MINERVA, $a_{t-1} \in \mathbb{R}^d$ and $o_t \in \mathbb{R}^d$ denote the vector representation for action/relation at time $t - 1$ and observation/entity at time $t$, respectively, and $[;]$ denotes the vector concatenation.

For Multi-Hop, $R_b(s_T)$ denotes the terminal reward, which is 1 if the agent  arrives at a correct target entity at the end of search, 0 otherwise. The reward function is generalized by a reward shaping strategy, where $f(e_s, r_q, e_T)$ is a pre-trained scoring function. 

For CPL, $b_{e_t}$ denotes the sentence bag of current entity. Specifically, the action space for the Reasoner is defined as the union of the edges in the current KG and edges extracted from the text corpus.

\begin{table}[!htbp]
\centering
\caption{Comparison of RL-based path finding for knowledge graph reasoning; 
    [$\dagger$] \cite{xiong-etal-2017-deeppath};
    [$\diamond$] \cite{das-2017-minerva}; 
    [$\star$]\cite{lin-2018-multihop} ; 
    [$\ddagger$]\cite{Shen2018MWalkLT};
    [$\circ$] \cite{fu-2019-collaborative};}
\resizebox{1\textwidth}{!}{
\begin{tabular}{$l^l^l^l^l}
\cmidrule{1-5}
\rowstyle{\bfseries}%
Method & State $s_t$ & Action $a_t$ & Reward $\gamma$ & Policy Network \\
\cmidrule{1-5}
\multicolumn{2}{l}{\bfseries RL on static knowledge bases} & & & \\
\cmidrule{1-5}
DeepPath[$\dagger$] & $(e_t, e_q - e_t)$ & $\{r\}$ & Global 1 $e_t=e_q$ & FCN\\
MINERVA[$\diamond$] & $(e_t, e_s, r_q, e_q)$ & $\{(e_t, r, v)\}$ & $\mathbbm{1}\{e_t = e_q\}$ & $h_t = LSTM(h_{t-1}, [a_{t-1}; o_t])$ \\
Multi-Hop[$\star$] & $(e_t, (e_s, r_q))$ & $\{(r', e') |(e_t, r', e') \in \mathcal{G}\}$ & $R_b(s_T) + (1-R_b(s_T)) f (e_s, r_q, e_T)$ & $h_t = LSTM(h_{t-1}, a_{t-1})$\\
M-Walk[$\ddagger$] & $s_{t-1} \cup \{a_{t-1}, v_t, \mathcal{E}_{\mathcal{G}_{v_t}}, \mathcal{V}_{v_t} \}$ & $ \mathcal{E}_{\mathcal{G}_{v_t}} \cup \{STOP\}$ & $\mathbbm{1}\{e_t = e_q\}$ & GRU-RNN + FCN\\
CPL [$\circ$] Reasoner & $(e_s, r_q, h_t)$ & $\{\xi \in \mathcal{E}_{\mathcal{G}}\}$ & $\mathbbm{1}\{e_t = e_q\}$ & $h_t = LSTM(h_{t-1}, [r_{t}; e_t])$ \\
CPL [$\circ$] Extractor & $(b_{e_t}, e_t)$ & $\{(r', e')\}_{(e_t, r', e')} \in b_{e_t}$ & delayed from reasoner & PCNN-Att \\
\cmidrule{1-5}
\multicolumn{2}{l}{\bfseries RL on non-static knowledge bases} & & & \\
\cmidrule{1-5}
\textbf{MIRA} 
& $s^i \coloneqq h(\Phi(s_{s}^{i}), \Phi(s_{o}^{i}))$

& $A^i \overset{\triangle}{=} p_s^i \cup p_o^i$
& $\mathbbm{1}\left\{\bigcup_{r \in c_s^{i+1}} N(r) \cap \bigcup_{r \in c_o^{i+1}} N(r)\right\}$
& FCN with Action-masking
\end{tabular}
}
\label{tab:scoring_fncs}
\end{table}

\section{Competitors - Adaptions}
\label{appendix:competitors}
\textbf{TNTComplex. } Note that the formulation of the loss presented in \cite{Lacroix2020Tensor} suits only to queries of the type $(subject, predicate, ?, time)$. As in our work, we focus on the relational prediction task (i.e., we want to infer the predicate), we slightly modify this loss function. For each of the train tuples (i, j, k, l), we define the loss function along the relational tube of the 4-order tensor. Hence, we get:

\begin{equation}
    \Tilde{l}(\hat{X}; (i,j,k,l)) = - \hat{X}_{i,j,k,l} + \log \left(\sum_{j'} exp(\hat{X}_{i,j',k,l})\right)
\end{equation}

\textbf{DE-TransE, DE-DistMult, DE-SimplE. }
By including the temporal information for a pair (v,t), where  $v \in \mathcal{V}, t \in \mathcal{T}$, the method yields a vector $z_v$ in a $d$-dimensional space. The scoring function underneath stays the same for the various methods.
For DE-TransE, we get $\phi(v,r,u) = - \|z_v + z_r - z_u\|$, for DE-DistMult $\phi(v,r,u) = \langle z_v, z_r, z_u\rangle$ and for DE-SimplE $\phi(v,r,u) = \left[ \langle z_v, z_r, z_u \rangle + \langle z_u, z_{r^{-1}}, z_v \rangle \right] / 2$.
